# Supplementary material for: FetchAid: Making Parcel Lockers More Accessible to Blind and Low Vision People With Deep-learning Enhanced Touchscreen Guidance, Error-Recovery Mechanism, and AR-based Search Support
Source: arXiv:2402.15723 source file (2024-02-24)
Supplement: Supplementary file 1 [file alg1.tex]

\begin{algorithm}
\footnotesize
 Point $A$: Finger's touching point\;
 Point $B$: The center point of the target button\;
 Polygon $R$: The geometric center of the target button’s learned boundary\;
 $d_x$: The distance from point $A$ to $B$ on the $x$ axis\;
 $d_y$: The distance from point $A$ to $B$ on the $y$ axis\;
 $success \ message$: ``fetch your package '' if the target is the ``Fetch Package'' button, else ``return to homepage''\;
 \While{detecting}{
  \eIf{$A$ is completely inside $R$}{
    $voice \ feedback$ = ``Please tap to'' + $success \ message$\;
  }{
      \eIf{$A$ is not bounded by $R$ on $x$ axis}{
              \eIf{$d_x$ > 0}{
               $DIR_x$ = ``left''\;
               }{
               $DIR_x$ = ``right''\;
              }
          }{
            $DIR_x$ = ``''\;
          }
      
      \eIf{$A$ is not bounded by $R$ on $y$ axis}{
          \eIf{$d_y$ > 0}{
           $DIR_y$ = ``up''\;
           }{
           $DIR_x$ = ``down''\;
          }
      }{
      $DIR_y$ = ``''\;
      }
      
      \eIf{$|d_x| < 40 \ cm \text{ or } |d_y| < 40 \ cm$}{
           $voice \ feedback$ = ``Please move'' + $DIR_x$ + $DIR_y$ + ``slowly''\;
           }{
           $voice \ feedback$ = ``Please move'' + $DIR_x$ + $DIR_y$\;
          }
  }
 }
 \caption{Voice Feedback Logic for Touchscreen Operation}
 \label{algorithm: Voice Feedback Logic for Touchscreen Operation}
\end{algorithm}
