# Supplementary material for: FetchAid: Making Parcel Lockers More Accessible to Blind and Low Vision People With Deep-learning Enhanced Touchscreen Guidance, Error-Recovery Mechanism, and AR-based Search Support
Source: arXiv:2402.15723 source file (2024-02-24)
Supplement: Supplementary file 2 [file alg2.tex]

\begin{algorithm}
\footnotesize
Point $A$: The center of the mobile phone\;
Point $B$: The center of the target compartment\;
$d_x$: The distance from $A$ to $B$ on $x$-axis\;
$d_y$: The distance from $A$ to $B$ on $y$-axis\;
 \While{detecting}{
 \eIf{ $|d_x| \leq 20 \ cm \text{ and } |d_y| \leq 10 \ cm$}{
     $voice \ feedback$ = ``You have reached the specified location''\;
 }{
   \eIf{
   $|d_x| \leq 20 \ cm$
   }{
       \eIf{$d_y \ > 0$}{
           $DIR_y$ = ``up''\;
           If $d_y \ > 45 \ cm$, then the \textit{reminder} voice feedback will be called once: ``The compartment is above, please reach out and touch.''
       }{
           $DIR_y$ = ``down''\;
           If $d_y \ < -65 \ cm$, then the \textit{reminder} voice feedback will be called once: ``The compartment is at your feet. Please bend down or squat down to touch it.''
       }
       \eIf{$|d_y| \leq 20$}{
       $voice \ feedback$ = ``Please move'' + $DIR_y$\ + ``slowly'';
       }{
       $voice \ feedback$ = ``Please move'' + $DIR_y$\;
       }
   }{
       \eIf{$d_x > 0$}{
       $DIR_x$ = ``left''\;
       }{
       $DIR_x$ = ``right''\;
       }
       \eIf{$|d_x| \leq 40$}{
       $voice \ feedback$ = ``Please move'' + $DIR_x$\ + ``slowly'';
       }{
       $voice \ feedback$ = ``Please move'' + $DIR_x$\;
       }
   }
 }
 }
 \caption{Voice Feedback Logic for Open Door Searching}
 \label{algorithm: Voice Feedback Logic for Open Door Searching}
\end{algorithm}
